# Supplementary material for: Adversarial Feature Matching for Text Generation
Source: arXiv:1706.03850 source file (2017-11-18)
Supplement: Supplementary file 1 [file suppl.pdf]

# A. Additional results

## A.1. RNN specifications

We leverage a LSTM RNN for our generator. Each LSTM unit has a cell containing a state $\boldsymbol{c}_t$ at time $t$. Reading or writing the memory unit is controlled through sigmoid gates, namely, input gate $\boldsymbol{i}_t$, forget gate $\boldsymbol{g}_t$, and output gate $\boldsymbol{o}_t$. The hidden units $\boldsymbol{h}_t$ are updated as follows:

$$\boldsymbol{i}_t = \sigma(\mathbf{W}_i \boldsymbol{y}_{t-1} + \mathbf{U}_i \boldsymbol{h}_{t-1} + \mathbf{C}_i \boldsymbol{z}) \quad (9)$$
$$\boldsymbol{g}_t = \sigma(\mathbf{W}_g \boldsymbol{y}_{t-1} + \mathbf{U}_g \boldsymbol{h}_{t-1} + \mathbf{C}_g \boldsymbol{z}) \quad (10)$$
$$\boldsymbol{o}_t = \sigma(\mathbf{W}_o \boldsymbol{y}_{t-1} + \mathbf{U}_o \boldsymbol{h}_{t-1} + \mathbf{C}_o \boldsymbol{z}) \quad (11)$$
$$\tilde{\boldsymbol{c}}_t = \tanh(\mathbf{W}_c \boldsymbol{y}_{t-1} + \mathbf{U}_c \boldsymbol{h}_{t-1} + \mathbf{C}_c \boldsymbol{z}) \quad (12)$$
$$\boldsymbol{c}_t = \boldsymbol{g}_t \odot \boldsymbol{c}_{t-1} + \boldsymbol{i}_t \odot \tilde{\boldsymbol{c}}_t \quad (13)$$
$$\boldsymbol{h}_t = \boldsymbol{o}_t \odot \tanh(\boldsymbol{c}_t) \,, \quad (14)$$

where $\sigma(\cdot)$ denotes the logistic sigmoid function, and $\odot$ represents the element-wise multiply operator (Hadamard product). $\mathbf{W}_{\{i,g,o,c\}}, \mathbf{U}_{\{i,g,o,c\}}$, $\mathbf{C}_{\{i,g,o,c\}}$, $\mathbf{V}$ and $\mathbf{C}$ are the set of parameters. Note that $\boldsymbol{z}$ is used as an explicit input at each time step of the LSTM to guide the generation of $\tilde{s}$. Another remark is that all the randomness in the generator come from $z$. The synthetic sentence $\tilde{s}$ is deterministically obtained given $z$.

## A.2. Universality of the embedded kernel

In below we consider the universality of a kernel defined on the input space $\mathcal{X}$, constructed by a universal kernel on feature space $\mathcal{F}$.

**Proposition 1.** *Suppose a continuous universal kernel $k : \mathcal{F} \times \mathcal{F} \to \mathbb{R}$ is a universal kernel. If a space $\mathcal{X}$ has a continuous bijective mapping $\lambda : \mathcal{X} \to \mathcal{F}$, the composed kernel $\tilde{k} : \mathcal{X} \times \mathcal{X} \to \mathbb{R}$, such that for $\forall x, x' \in \mathcal{X}$, $\tilde{k}(x, x') = k(f(x), f(x'))$ is a universal kernel define on $\mathcal{X}$.*

*Proof.* Denote $\mathbb{N}_n = \{1, 2, \cdots, n\}$. Since $k$ is a universal kernel, from Micchelli et al. (2006), $k$ is continuous and its RKHS $\mathcal{H}$ is dense in $C(\mathcal{F}) \triangleq \{g : \mathcal{F} \to \mathbb{R} | g\text{continuous}\}$, *i.e.*, for any $n$ points $\{f_i\}_{i \in \mathbb{N}_n} \in \mathcal{F}$, for $\forall g \in C(\mathcal{F})$, there exists $a_i : i \in \mathbb{N}_n$ that

$$g(\cdot) = \sum_{i \in \mathbb{N}_n} a_i k(f_i, \cdot) \,, \quad (15)$$

where $k(f_i, \cdot) \in \mathcal{H}$. This is known as the *universal approximation* property. Since $\lambda$ is a bijective function, consider any $\{x_i\}_{i \in \mathbb{N}_n} \in \mathcal{X}$. By construction, for $\forall h \in C(\mathcal{X}) \triangleq h : \mathcal{X} \to \mathbb{R} | h\text{continuous}$, consider $g = h \circ \lambda^{-1}$, from (**??**) we have

$$h(x) = h(\lambda^{-1}(\lambda(x))) = g(\lambda(x)) \quad (16)$$
$$= \sum_{i \in \mathbb{N}_n} a_i k(\lambda(x_i), \cdot) = \sum_{i \in \mathbb{N}_n} a_i \tilde{k}(x_i, \cdot) \,. \quad (17)$$

Hence the $\tilde{k}$ is a universal kernel. □

## A.3. Alternative upper bound objective

In this subsection we show that (5) corresponds to an upper bound of the JSD between two Gaussian distribution.

*Proof.* The KL divergence $D_{KL}(p||q)$ between two multivariate Gaussian distribution $p(x) \sim \mathcal{N}(\boldsymbol{\mu}, \boldsymbol{\Sigma})$ and $q(x) \sim \mathcal{N}(\tilde{\boldsymbol{\mu}}, \tilde{\boldsymbol{\Sigma}})$ is given by

$$D_{KL}(p||q) = \frac{1}{2}\Big[\text{tr}(\tilde{\boldsymbol{\Sigma}}^{-1}\boldsymbol{\Sigma}) + \log \frac{|\tilde{\boldsymbol{\Sigma}}|}{\boldsymbol{\Sigma}} + \quad (18)$$
$$+ (\tilde{\boldsymbol{\mu}} - \boldsymbol{\mu})^T (\tilde{\boldsymbol{\Sigma}}^{-1})(\tilde{\boldsymbol{\mu}} - \boldsymbol{\mu}) - d\Big] \,. \quad (19)$$

We first start with a proposition.

**Proposition 2.** *Assume three arbitrary valid continuous density functions $p, q, r$ has probability measures over a domain $\mathcal{X}$, we have that $D_{KL}(p||q) + D_{KL}(p||r) \geq D_{KL}(p||(q + r)/2)$.*

The proof is as follows.

$$D_{KL}(p||q) + D_{KL}(p||r) \quad (20)$$
$$= \int -p(x) \log \frac{q(x)}{p(x)} + \log \frac{r(x)}{p(x)} \quad (21)$$
$$<= \int -p(x) \log \frac{[q(x) + r(x)]/2}{p(x)} \quad (22)$$
$$= D_{KL}(p||(q + r)/2) \,. \quad (23)$$

From (**??**) and (**??**), following the definition of JSD, we have

$$JSD(p||q) \quad (24)$$
$$= D_{KL}\Big(p\Big|\Big|\frac{p+q}{2}\Big) + D_{KL}\Big(q\Big|\Big|\frac{p+q}{2}\Big) \quad (25)$$
$$<= D_{KL}(p||p) + D_{KL}(p||q) \quad (26)$$
$$+ D_{KL}(q||q) + D_{KL}(q||p) \quad (27)$$
$$= \frac{1}{2}\Big[\text{tr}(\tilde{\boldsymbol{\Sigma}}^{-1}\boldsymbol{\Sigma} + \boldsymbol{\Sigma}^{-1}\tilde{\boldsymbol{\Sigma}})$$
$$+ (\tilde{\boldsymbol{\mu}} - \boldsymbol{\mu})^T (\tilde{\boldsymbol{\Sigma}}^{-1} + \boldsymbol{\Sigma}^{-1})(\tilde{\boldsymbol{\mu}} - \boldsymbol{\mu}) - 2d\Big] \,. \quad (28)$$

Therefore, (5) is an upper bound for $JSD(p||q)$. Directly minimizing $JSD(p||q)$ is hard, however (5) is more tractable. □

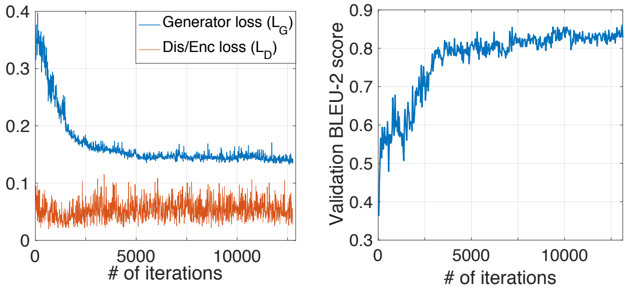


*Figure 4.* Left: learning curve for TextGAN. Right: validation BLEU-2 score.

### A.4. VAE and KL divergence annealing

In VAE we optimize the lower bound objective below.

$$\mathcal{L} = \mathbb{E}_{q(z|x)} \log p(x|z) + \alpha \mathbb{E}_{q(z|x)} [\log p(z) - \log q(z|x)] \,,$$

where $\alpha$ is a scaling parameter. We observed that directly minimizing the above objective with $\alpha = 1$ would fail to converge. Thus we train the VAE under an annealing scheme, where $\alpha_t$ is set to be $\min(t/50,000, 1)$ and $t$ is the number of iterations that has been performed.

### A.5. Feature matching results

The covariance matrices of real features $\boldsymbol{f}$ and synthetic features $\tilde{\boldsymbol{f}}$ are shown Figure **??**. Each of the covariance matrices is computed over 2,000 data points. Learning curves are shown in Figure **??**.

### A.6. Experimental setup

To accelerate convergence, we begin each run with a warm-up training. Specifically, This warm-up includes: (*i*) using a mean matching objective for the generator loss, *i.e.*, $||\mathbb{E}\boldsymbol{f} - \mathbb{E}\tilde{\boldsymbol{f}}||^2$, as in Salimans et al. (2016); (*ii*) trimming the generated sentences if the length exceeds 15, by removing words afterwards. For MMD Gaussian kernel, we set the bandwidth parameters as $[10, 15, 20, 25, 30]$ in our experiments. The $L$ used in soft-argmax is $10,000$. The $\lambda_r$ and $\lambda_m$ are set to be $0.01$ and $0.001$. The activation function employed in discriminator/encoder is hyperbolic tangent function. We also utilized several other training techniques in order to stabilize training, including soft-labeling (Salimans et al., 2016) and batch normalization (Ioffe & Szegedy, 2015). For soft-labeling the discriminator is constraint to maximally assign 0.99 and minimally assign 0.01 for the probability of being from real data. The batch normalization is added on the CNN output before activation function. In practice we find batchnorm does not provide significant performance benefits.

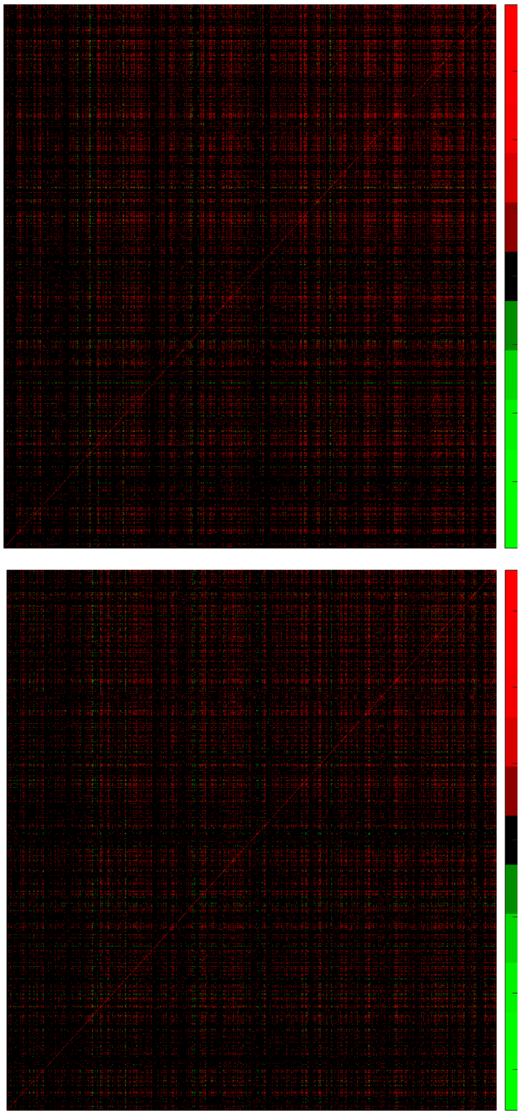

*Figure 5.* Covariance matching. Upper: synthetic features covariance. Lower: real features covariance.
